# Supplementary material for: Shear thinning in dilute and semidilute solutions of polystyrene and DNA
Source: arXiv:1710.08050 ancillary file (2018-05-06)
Supplement: Supplementary file 1 [file 1710.08050v2_SM.pdf]

# Supplementary material for: Shear thinning in dilute and semidilute solutions of polystyrene and DNA

Sharadwata Pan
*IITB-Monash Research Academy, Indian Institute of Technology Bombay, Powai, Mumbai - 400076, India*
*Department of Chemical Engineering, Indian Institute of Technology Bombay, Powai, Mumbai - 400076, India and*
*Department of Chemical Engineering, Monash University, Melbourne, VIC 3800, Australia*

Duc At Nguyen
*Department of Chemical Engineering, Monash University, Melbourne, VIC 3800, Australia*

B. Dünweg
*Department of Chemical Engineering, Monash University, Melbourne, VIC 3800, Australia*
*Max Planck Institute for Polymer Research, Ackermannweg 10, 55128 Mainz, Germany and*
*Condensed Matter Physics, TU Darmstadt, Hochschulstraße 12, 64289 Darmstadt, Germany*

P. Sunthar
*Department of Chemical Engineering, Indian Institute of Technology Bombay, Powai, Mumbai - 400076, India and*
*IITB-Monash Research Academy, Indian Institute of Technology Bombay, Powai, Mumbai - 400076, India*

T. Sridhar and J. Ravi Prakash*
*Department of Chemical Engineering, Monash University, Melbourne, VIC 3800, Australia and*
*IITB-Monash Research Academy, Indian Institute of Technology Bombay, Powai, Mumbai - 400076, India*
(Dated: March 9, 2018)

## I. DNA SAMPLE PREPARATION

The DNA samples were dissolved in a solvent containing 10 mM Tris (#T1503, Sigma-Aldrich), 1 mM EDTA (#E6758, Sigma-Aldrich) and 0.5 M NaCl (#S5150, Sigma-Aldrich), which was also used for preparing subsequent dilutions. The solvent has a viscosity of 1.01 mPa.s at 20°C, which is approximately equal to the viscosity of water. For linear genomic DNAs from T4 and $\lambda$ phages, with anticipated purity of high orders, concentrations of 0.24 mg/ml and 0.5 mg/ml, respectively, were used, as specified by the companies. For the 25 kbp linear DNA, the concentration of DNA (0.441 mg/ml) was determined by both UV-VIS spectrophotometry (#UV-2450, Shimadzu) and agarose gel electrophoresis, the latter by comparing with a standard DNA marker (#N0468L, New England Biolabs). The $A_{260}/A_{280}$ and $A_{260}/A_{230}$ ratios were 1.92 and 2.1 respectively, the latter indicating absence of organic reagents like phenol, chloroform etc. [1], and suggesting an overall good quality of the DNA sample, as noted earlier by Laib et al. [2]

## II. SHEAR RHEOMETRY

A Contraves Low Shear 30 rheometer (1T/1T – cup and bob; shear rate $\dot{\gamma}$ range: 0.01–100 $s^{-1}$; temperature sensitivity: ± 0.1°C) has been used to obtain all the shear viscosity measurements reported in the present work. The measuring principles underlying the Contraves rheometer have been detailed in a recent study [3]. The rheometer was calibrated with Newtonian Standards (silicone oils) of known viscosities (around 10, 100 and 1000 mPa-s at 20°C), and the zero error adjustment was carried out as described earlier in Ref. [4]. Values obtained fall within 5% of the company specified values. A continuous shear ramp was avoided, and to avert the problem of aggregation of long DNA chains, $\lambda$ and T4 DNA (at their maximum concentrations) were kept at 65°C for 10 minutes and instantly put into ice for 10 minutes [3, 5]. A manual delay of 30 seconds was applied at each shear rate to allow the DNA chains to relax to their equilibrium state and the sample was equilibrated for 30 minutes at each temperature. Some typically observed relaxation times are given in Table I of Ref. [4]. We have also established that the measured viscosity does not depend on rheometer geometry in the range of shear rates employed (in terms of the 'gap' between the cup and the bob), by measuring the viscosity of T4 DNA at two different gaps at two different temperatures, as elaborated in our earlier work [6].

## III. DILUTE SOLUTION ZERO SHEAR RATE VISCOSITY

### A. DNA samples

Pan et al. [6] have previously determined the zero shear rate solution viscosity, $\eta_0$, for dilute 25 kbp and T4 DNA

* Corresponding author: ravi.jagadeeshan@monash.edu

TABLE I. Steady state zero shear rate viscosities, $\eta_0$ (mPa.s) for 25 kbp, $\lambda$-phage, and T4 DNA at various concentrations $c$ (mg/ml) and temperatures $T$ (°C) in the dilute regime ($0 < c/c^* < 1$).

25 kbp

| $c$ | $T$ | $c/c^*$ | $\eta_0$ |
|---|---|---|---|
| 0.112 | 15 | 0.91 | 2.95 ± 0.01 |
| 0.07 | 15 | 0.57 | 1.76 ± 0.01 |
| | 18 | 0.74 | 1.75 ± 0.01 |
| | 21 | 0.85 | 1.72 ± 0.01 |
| | 25 | 0.97 | 1.58 ± 0.02 |
| 0.0441 | 15 | 0.36 | 1.53 ± 0.01 |
| | 18 | 0.46 | 1.49 ± 0.01 |
| | 21 | 0.54 | 1.43 ± 0.01 |
| | 25 | 0.61 | 1.31 ± 0.01 |
| | 30 | 0.7 | 1.27 ± 0.01 |
| | 35 | 0.76 | 1.2 ± 0.01 |
| 0.028 | 15 | 0.23 | 1.38 ± 0.01 |
| | 18 | 0.29 | 1.31 ± 0.01 |
| | 21 | 0.34 | 1.25 ± 0.01 |
| | 25 | 0.39 | 1.15 ± 0.01 |
| | 30 | 0.44 | 1.09 ± 0.01 |
| | 35 | 0.48 | 1.01 ± 0.01 |
| 0.0175 | 15 | 0.14 | 1.29 ± 0.01 |
| | 18 | 0.18 | 1.2 ± 0.01 |
| | 21 | 0.21 | 1.14 ± 0.01 |
| | 25 | 0.24 | 1.05 ± 0.01 |
| | 30 | 0.28 | 0.98 ± 0.01 |
| | 35 | 0.3 | 0.9 ± 0.01 |

$\lambda$-phage

| $c$ | $T$ | $c/c^*$ | $\eta_0$ |
|---|---|---|---|
| 0.05 | 15 | 0.56 | 2.35 ± 0.02 |
| | 18 | 0.78 | 2.14 ± 0.02 |
| | 21 | 0.93 | 2.04 ± 0.02 |
| 0.0315 | 15 | 0.35 | 1.88 ± 0.01 |
| | 18 | 0.49 | 1.75 ± 0.01 |
| | 21 | 0.58 | 1.73 ± 0.01 |
| | 25 | 0.68 | 1.61 ± 0.01 |
| | 30 | 0.77 | 1.52 ± 0.01 |
| | 35 | 0.85 | 1.39 ± 0.01 |
| 0.02 | 15 | 0.22 | 1.52 ± 0.01 |
| | 18 | 0.31 | 1.42 ± 0.01 |
| | 21 | 0.37 | 1.36 ± 0.01 |
| | 25 | 0.43 | 1.28 ± 0.01 |
| | 30 | 0.49 | 1.15 ± 0.01 |
| | 35 | 0.54 | 1.04 ± 0.01 |
| 0.0125 | 15 | 0.14 | 1.39 ± 0.01 |
| | 18 | 0.2 | 1.28 ± 0.01 |
| | 21 | 0.23 | 1.22 ± 0.01 |
| | 25 | 0.27 | 1.15 ± 0.01 |
| | 30 | 0.3 | 1.04 ± 0.01 |
| | 35 | 0.34 | 0.94 ± 0.01 |
| 0.008 | 15 | 0.09 | 1.29 ± 0.01 |
| | 18 | 0.13 | 1.21 ± 0.01 |
| | 21 | 0.15 | 1.13 ± 0.01 |
| | 25 | 0.17 | 1.06 ± 0.01 |
| | 30 | 0.2 | 0.96 ± 0.01 |
| | 35 | 0.22 | 0.87 ± 0.01 |

T4 DNA

| $c$ | $T$ | $c/c^*$ | $\eta_0$ |
|---|---|---|---|
| 0.038 | 15 | 0.79 | 5.38 ± 0.13 |
| 0.023 | 15.7 | 0.58 | 2.43 ± 0.01 |
| | 17.3 | 0.72 | 2.33 ± 0.01 |
| | 19.4 | 0.85 | 2.23 ± 0.01 |
| 0.015 | 15.7 | 0.38 | 1.96 ± 0.01 |
| | 17.3 | 0.47 | 1.86 ± 0.01 |
| | 19.4 | 0.56 | 1.79 ± 0.01 |
| | 22 | 0.65 | 1.68 ± 0.01 |
| | 24.5 | 0.71 | 1.6 ± 0.01 |
| 0.0094 | 15 | 0.2 | 1.51 ± 0.01 |
| | 20 | 0.36 | 1.48 ± 0.01 |
| | 25 | 0.39 | 1.43 ± 0.01 |
| | 30 | 0.52 | 1.4 ± 0.01 |
| | 35 | 0.59 | 1.37 ± 0.01 |
| 0.0059 | 15 | 0.12 | 1.36 ± 0.01 |
| | 20 | 0.23 | 1.29 ± 0.01 |
| | 25 | 0.25 | 1.22 ± 0.01 |
| | 30 | 0.33 | 1.16 ± 0.01 |
| | 35 | 0.37 | 1.09 ± 0.01 |
| 0.0038 | 15 | 0.08 | 1.27 ± 0.01 |
| | 20 | 0.14 | 1.18 ± 0.01 |
| | 25 | 0.15 | 1.09 ± 0.01 |
| | 30 | 0.21 | 1.02 ± 0.01 |
| | 35 | 0.23 | 0.96 ± 0.01 |

solutions by least-square fitting the values of viscosity in the plateau region of very low shear rates, across a range of temperatures and concentrations below $c^*$, and extrapolating to zero shear rate. For details, see the supplementary information in Ref. [6]. The zero shear rate solution viscosity for $\lambda$-phage DNA has been determined here using the same procedure. Data for the all the three DNA samples, for various values of $c/c^*$ and $T$, are displayed in Table I (with the data for the 25 kbp and T4 DNA solutions reproduced here from Ref. [6]).

Since the viscosity of the solvent for DNA solutions (containing 10 mM Tris, 1 mM EDTA, and 0.5 M NaCl), is almost identical to the viscosity of water at 20°C, the solvent viscosity at any other temperature was considered to be equal to that of the viscosity of water at that temperature. Water viscosities reported at https://www.thermexcel.com/english/tables/eau_atm.htm were used since they are tabulated at intervals of 1°C, for an extended range of temperatures. Note that where temperatures coincide, these values of viscosity are identical to those reported by Howe et al. [8]. Values of viscosity at intermediate temperatures were obtained by linear interpolation between the nearest two temperatures. The polymer contribution to steady state zero shear rate viscosity, $\eta_{p0} = \eta_0 - \eta_s$, for all the dilute and semidilute DNA solutions, can then be obtained.

### B. Polystyrene samples

The steady state solution shear viscosity, $\eta$, was measured by Hua and Wu [7] for solutions of four different molecular weights of polystyrene in dioctyl phthalate (denoted PS1 to PS4), for a range of temperatures. The zero shear rate viscosities $\eta_0$ at each temperature have been extracted (as in the case of DNA solutions) by least-square fitting the values of viscosity in the plateau region of very low shear rates, and extrapolating to zero shear rate. The procedure for determining the solvent viscosity $\eta_s$ as a function of temperature for the dioctyl phthalate solutions has been described in Appendix A of the main paper. Using these values, the polymer contribution to steady state zero shear rate viscosity, $\eta_{p0} = \eta_0 - \eta_s$, has been obtained for all the polystyrene solutions, and is displayed in Table II for various values of $c/c^*$ (calculated as described in Appendix A of the main paper) and $T$.

TABLE II. Polymer contribution to steady state zero shear rate viscosity, $\eta_{p,0}$, at various temperatures, for the dilute polystyrene samples PS1 to PS4 used in Ref. [7].

| Sample | $M$ ($\times 10^6$ g/mol) | $c$ (g/ml) | $T$ (°C) | $c/c^*$ | $\eta_{p,0}$ (mPa.s) |
|---|---|---|---|---|---|
| PS1 | 0.55 | 0.0046 | 22 | 0.223 | 16.1 ± 0.1 |
| | | | 25 | 0.239 | 13.8 ± 0.1 |
| | | | 35 | 0.283 | 9.9 ± 0.1 |
| | | | 45 | 0.318 | 5.6 ± 0.04 |
| PS2 | 0.68 | 0.0048 | 22 | 0.266 | 23.9 ± 0.3 |
| | | | 25 | 0.287 | 18.3 ± 0.4 |
| | | | 35 | 0.344 | 11.4 ± 0.01 |
| | | | 45 | 0.390 | 7.8 ± 0.2 |
| PS3 | 0.93 | 0.0054 | 22 | 0.350 | 31.9 ± 0.9 |
| | | | 25 | 0.383 | 24.3 ± 0.1 |
| | | | 35 | 0.469 | 15.5 ± 0.2 |
| | | | 45 | 0.536 | 10.8 ± 0.1 |
| PS4 | 2.0 | 0.0028 | 22 | 0.269 | 27.9 ± 0.4 |
| | | | 25 | 0.305 | 20.6 ± 0.2 |
| | | | 35 | 0.395 | 13.2 ± 0.2 |
| | | | 45 | 0.464 | 9.9 ± 0.01 |

## IV. SEMIDILUTE SOLUTION ZERO SHEAR RATE VISCOSITY

### A. DNA samples

The steady state shear viscosities $\eta$ of the three DNA solutions were measured for a variety of concentrations in the semidilute regime and across a temperature range of 15–35°C. Examples of the dependence of measured solution shear viscosity on shear rate $\dot{\gamma}$ are displayed in Figs. 1 (a) and (b). The former displays the viscosity of 25 kbp DNA at a fixed concentration $c = 0.441$ mg/ml and at various temperatures ranging from $T = 15.8$ to 44.6°C. Since $c^*$ varies with temperature, this corresponds to values of $c/c^*$ ranging from 2.12 to 8.65 (see Table III), all of which are in the semidilute regime. In Fig. 1 (b), the dependence of $\eta$ on $\dot{\gamma}$ of T4 DNA at a fixed temperature $T = 25$°C, is shown at various concentrations, varying from 0.059 to 0.214 mg/ml. This corresponds to a $c/c^*$ range of 2.98 to 10.82, as displayed in Table III. As in the case of dilute polymer solutions, the zero shear rate viscosity $\eta_0$ was determined by least-square fitting the values of viscosity in the plateau region of very low shear rates, at each temperature and concentration, and extrapolating to zero shear rate. Details are given in our earlier work [4]. Values obtained in this way for the three DNA samples, across the range of concentrations and temperatures, are displayed in Table III, reproduced here from Ref. [4].

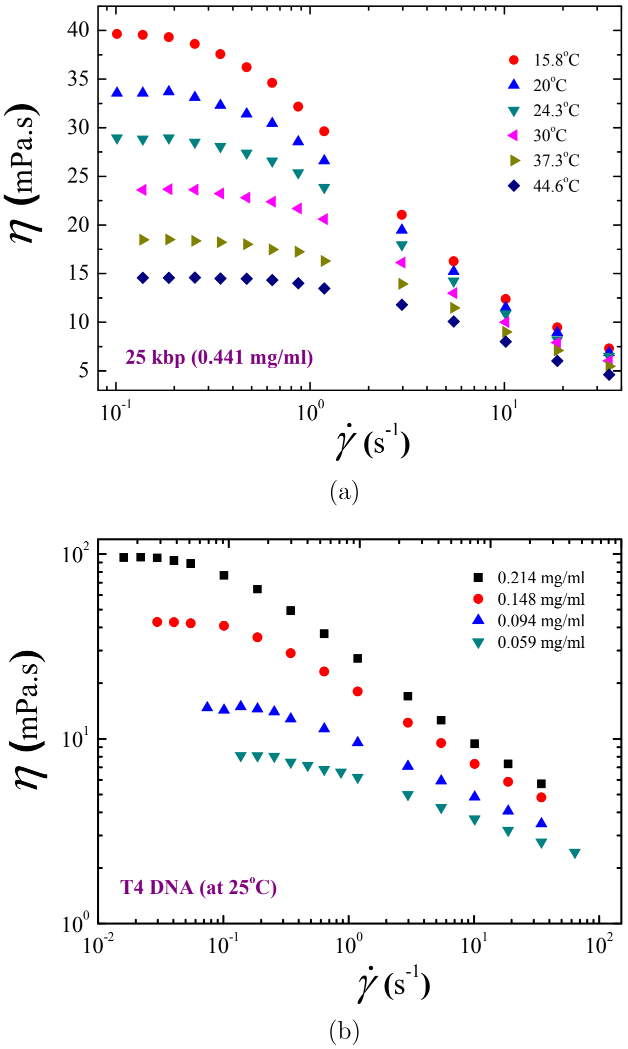


FIG. 1. (a) Shear rate dependence of the steady state semidilute solution shear viscosity for 25 kbp DNA at a fixed absolute concentration for different temperatures. (b) Shear rate dependence of the steady state shear semidilute solution viscosity for T4 DNA at a fixed temperature for different absolute concentrations.

### B. Polystyrene samples

The steady state shear viscosities $\eta$ were measured for the polystyrene solutions PS1.1M and PS15.4M across a range of concentrations and temperatures. Values of $\eta_{p,0}$ for these solutions have been determined identically as in the case of all the other solutions considered here, and are displayed in Table IV.

## V. DEPENDENCE OF RELAXATION TIME $\lambda_\eta$ ON TEMPERATURE

The temperature dependence of $\lambda_\eta$ has been discussed in the main paper, with data indicating a linear relationship between $\lambda_\eta$ and $1/T$. Additional data displaying

TABLE III. Steady state zero shear rate viscosities (mPa.s) for 25 kbp, $\lambda$-phage, and T4 DNA at various concentrations, $c$ (mg/ml) and temperatures, $T$ (°C) in the semidilute regime ($1 \leq c/c^* \leq 10$).

| 25 kbp | | | |
|---|---|---|---|
| $c$ | $T$ | $c/c^*$ | $\eta_0$ |
| 0.441 | 15.8 | 3.9 | 39.3 ± 0.5 |
| | 20 | 5.13 | 33.5 ± 0.2 |
| | 24.3 | 6.04 | 28.8 ± 0.2 |
| | 30 | 7.0 | 23.5 ± 0.2 |
| | 37.2 | 7.88 | 18.4 ± 0.1 |
| | 44.6 | 8.65 | 14.5 ± 0.1 |
| 0.364 | 15.8 | 3.22 | 20.4 ± 0.1 |
| | 20 | 4.23 | 17.7 ± 0.1 |
| | 24.3 | 4.99 | 15.5 ± 0.1 |
| | 30 | 5.78 | 12.8 ± 0.1 |
| | 37.2 | 6.5 | 10.5 ± 0.1 |
| | 44.6 | 7.14 | 8.5 ± 0.01 |
| 0.315 | 15.8 | 2.79 | 14.7 ± 0.04 |
| | 20 | 3.66 | 12.7 ± 0.1 |
| | 24.3 | 4.32 | 11.2 ± 0.01 |
| | 30 | 5 | 9.3 ± 0.03 |
| | 37.2 | 5.63 | 7.7 ± 0.05 |
| | 44.6 | 6.18 | 6.6 ± 0.05 |
| 0.112 | 18 | 1.18 | 2.7 ± 0.02 |
| | 21 | 1.37 | 2.5 ± 0.01 |
| | 25 | 1.56 | 2.3 ± 0.02 |
| | 30 | 1.78 | 2 ± 0.02 |
| | 35 | 1.93 | 1.8 ± 0.01 |
| 0.07 | 30 | 1.11 | 1.5 ± 0.01 |
| | 35 | 1.21 | 1.5 ± 0.01 |

| $\lambda$ DNA | | | |
|---|---|---|---|
| $c$ | $T$ | $c/c^*$ | $\eta_0$ |
| 0.315 | 21 | 5.83 | 61.4 ± 1.05 |
| | 25 | 6.85 | 57.9 ± 0.9 |
| 0.2 | 15 | 2.25 | 16 ± 0.1 |
| | 21 | 3.7 | 14.6 ± 0.3 |
| | 25 | 4.35 | 12.3 ± 0.6 |
| | 30 | 4.88 | 11.3 ± 0.3 |
| | 35 | 5.41 | 10 ± 0.2 |
| 0.125 | 21 | 2.31 | 6.1 ± 0.1 |
| | 25 | 2.72 | 5.6 ± 0.2 |
| | 30 | 3.05 | 5 ± 0.1 |
| | 35 | 3.38 | 4.4 ± 0.1 |
| 0.08 | 21 | 1.48 | 3.4 ± 0.02 |
| | 25 | 1.74 | 3.1 ± 0.01 |
| | 30 | 1.95 | 2.8 ± 0.01 |
| | 35 | 2.16 | 2.5 ± 0.03 |
| 0.05 | 25 | 1.09 | 1.9 ± 0.01 |
| | 30 | 1.22 | 1.7 ± 0.01 |
| | 35 | 1.35 | 1.6 ± 0.02 |

| T4 DNA | | | |
|---|---|---|---|
| $c$ | $T$ | $c/c^*$ | $\eta_0$ |
| 0.148 | 15 | 3.08 | 55.9 ± 0.7 |
| | 18 | 4.93 | 50.7 ± 0.5 |
| | 21 | 6.14 | 46.7 ± 0.5 |
| | 25 | 7.48 | 42.5 ± 0.4 |
| | 30 | 8.22 | 37.1 ± 0.2 |
| | 35 | 9.52 | 32.5 ± 0.3 |
| 0.094 | 15 | 1.96 | 19.2 ± 0.6 |
| | 18 | 3.13 | 17.6 ± 0.4 |
| | 21 | 3.92 | 16.6 ± 0.1 |
| | 25 | 4.75 | 14.6 ± 0.3 |
| | 30 | 5.22 | 12.9 ± 0.2 |
| | 35 | 6.05 | 11.6 ± 0.2 |
| 0.059 | 15 | 1.23 | 10.2 ± 0.2 |
| | 18 | 1.97 | 9.6 ± 0.1 |
| | 21 | 2.46 | 8.9 ± 0.1 |
| | 25 | 2.98 | 8.1 ± 0.03 |
| | 30 | 3.28 | 7.3 ± 0.1 |
| | 35 | 3.79 | 6.6 ± 0.1 |
| 0.038 | 18 | 1.27 | 4.9 ± 0.2 |
| | 21 | 1.58 | 4.6 ± 0.2 |
| | 25 | 1.92 | 4.2 ± 0.2 |
| | 30 | 2.11 | 3.8 ± 0.2 |
| | 35 | 2.44 | 3.3 ± 0.05 |
| 0.023 | 22 | 1 | 2.1 ± 0.01 |
| | 24.5 | 1.1 | 2 ± 0.01 |

similar behaviour, at other concentrations, is shown in Figs. 2 for the three DNA and for the polystyrene solutions PS1.1M and PS15.4M, respectively.

## VI. DEPENDENCE OF DILUTE SOLUTION VISCOSITY ON SHEAR RATE

The steady state solution viscosity $\eta$ of the three DNA solutions was measured as a function of shear rate $\dot{\gamma}$ for a variety of concentrations in the dilute regime, and across a temperature range in the crossover regime from $\theta$ to good solvents (15–35°C). While the dependence of $\eta$ on $\dot{\gamma}$ at fixed concentration and at various temperatures is displayed in Figs. 3 (a), (c) and (e), the dependence at fixed temperature and various concentrations is shown in Figs. 3 (b), (d) and (f). The data presented in these figures is also given in tabular form in Tables V, VI and VII, so that they are readily available for comparison with any model predictions that may be made in the future for the shear thinning of dilute polymer solutions.

The general pattern of the viscosity curves is typical of the behaviour observed for polymer solutions, with a constant plateau region at low shear rates denoting Newtonian behaviour, followed by shear thinning at high shear rates. For each of the DNA, the viscosity can be seen to decrease with increasing temperature, at a fixed concentration. However, a change in the temperature does not appear to significantly affect the shear rate at which the onset of shear thinning occurs. On the other hand, at a fixed temperature, the viscosity increases with increasing concentration, and the increase in concentration appears to decrease the shear rate at which the onset of shear thinning occurs.

## VII. DEPENDENCE OF SEMIDILUTE SOLUTION VISCOSITY ON SHEAR RATE

Fig. 4 displays the dependence of the scaled viscosity $\eta_{\rm p}/\eta_{\rm p,0}$ on the shear rate $\dot{\gamma}$, for 25 kbp, $\lambda$-phage, and T4 DNA, while Fig. 5 displays the same dependence for the two polystyrene samples examined in this work, i.e., PS1.1M and PS15.4M, in the semidilute regime. As discussed in section IV, values of $\eta_0$ for all the samples have been determined identically as in the case of all the other

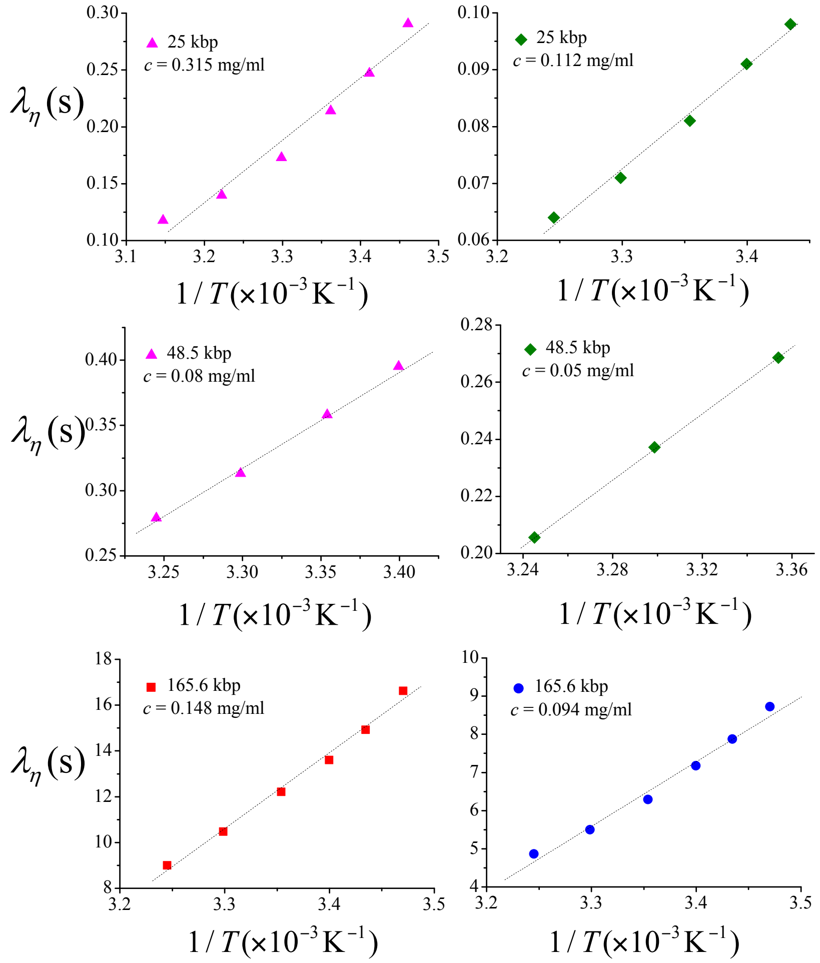


(a)

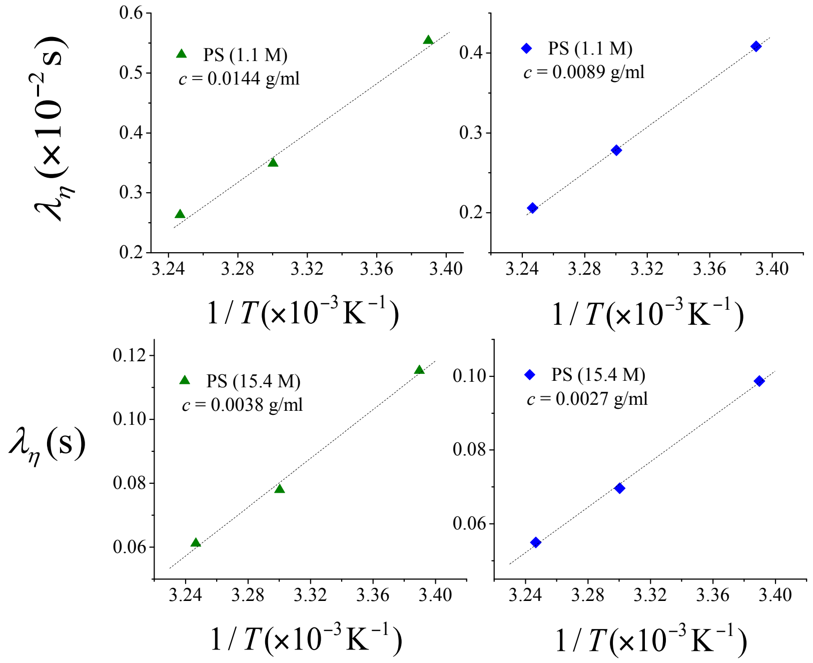


(b)

FIG. 2. Semidilute solution relaxation time $\lambda_\eta$ vs $1/T$ at a fixed concentration $c$ for (a) 25 kbp, 48.5 kbp, and 165.6 kbp DNA, and (b) polystyrene solutions PS1.1M and PS15.4M. The lines are the linear least squares fit to the data.

TABLE IV. Steady state zero shear rate viscosities (mPa.s) for polystyrene solutions PS1.1M and PS15.4M at various concentrations, $c$ (mg/ml) and temperatures, $T$ (°C) in the semidilute regime ($1 \leq c/c^* \leq 10$).

| PS1.1M | | | | PS15.4M | | | |
|---|---|---|---|---|---|---|---|
| $c$ (g/ml) | $T$ (°C) | $c/c^*$ (estimated) | $\eta_0$ (mPa.s) | $c$ (g/ml) | $T$ (°C) | $c/c^*$ (estimated) | $\eta_0$ (mPa.s) |
| | 22 | 2.59 | 1686.5 ± 1.3 | | 22 | 2.68 | 443.4 ± 2.8 |
| 0.036 | 30 | 3.19 | 980.8 ± 2.1 | 0.0098 | 30 | 4.50 | 291.7 ± 2.1 |
| | 35 | 3.48 | 721.6 ± 0.9 | | 35 | 5.33 | 223.6 ± 0.2 |
| | 22 | 1.62 | 505.6 ± 0.6 | | 22 | 1.67 | 196.9 ± 0.6 |
| 0.0225 | 30 | 1.99 | 308.2 ± 0.6 | 0.0061 | 30 | 2.80 | 133.6 ± 1.1 |
| | 35 | 2.18 | 238.6 ± 0.3 | | 35 | 3.32 | 105 ± 0.6 |
| | 22 | 1.04 | 240.4 ± 0.2 | | 22 | 1.04 | 139.3 ± 0.4 |
| 0.0144 | 30 | 1.27 | 153.7 ± 0.3 | 0.0038 | 30 | 1.75 | 91.7 ± 0.3 |
| | 35 | 1.39 | 118.3 ± 0.2 | | 35 | 2.07 | 72.3 ± 0.3 |
| | 22 | | | | 22 | < 1.0 | |
| 0.0089 | 30 | < 1.0 | | 0.0027 | 30 | 1.24 | 74 ± 0.1 |
| | 35 | | | | 35 | 1.47 | 58.3 ± 0.2 |

solutions considered here, and are displayed in Tables III and IV, for DNA and polystyrene, respectively. The 'raw' viscosity versus shear rate data presented in a scaled form in these figures is given in tabular form in Tables VIII, IX, X and XI for DNA, and Tables XII and XIII for polystyrene, so that they are readily available for comparison with any model predictions that may be made in the future for the shear thinning of semidilute polymer solutions.

Each of the subfigures in these plots corresponds to a different concentration, with the individual symbols in the subfigures representing different temperatures. All the displayed concentrations correspond to solutions in the semidilute regime, as can be confirmed from the values of $c/c^*$ listed in Tables III and IV. The reason the scaled viscosity appears to *increase* with temperature is because of the division of $\eta_{\rm p}$ by $\eta_{\rm p,0}$. While, as expected, $\eta_{\rm p}$ decreases with increasing temperature (see Fig. 1 for the behaviour of 25 kbp DNA), the shear rate dependence of $\eta_{\rm p}$ is more pronounced over the same range of shear rates, for solutions at a lower temperature.


[1] J. Sambrook and D. W. Russell. *Molecular Cloning: A Laboratory Manual (3rd edition.* Cold Spring Harbor Laboratory Press, USA, 2001.

[2] S. Laib, R. M. Robertson, and D. E. Smith. Preparation and characterization of a set of linear DNA molecules for polymer physics and rheology studies. *Macromolecules*, 39(12):4115–4119, 2006.

[3] Y. Heo and R. G. Larson. The scaling of zero-shear viscosities of semidilute polymer solutions with concentration. *J. Rheol.*, 49(5):1117–1128, 2005.

[4] S. Pan, D. A. Nguyen, P. Sunthar, T. Sridhar, and J. R. Prakash. Universal solvent quality crossover of the zero shear rate viscosity of semidilute DNA solutions. *J. Rheol.*, 58(2):339–368, 2014.

[5] K. Hsiao, C. Sasmal, J. R. Prakash, and C. M Schroeder. Direct observation of DNA dynamics in semidilute solutions in extensional flow. *J. Rheol.*, 61(1):151–167, 2017.

[6] S. Pan, D. Ahirwal, D. A. Nguyen, P. Sunthar, T. Sridhar, and J. R. Prakash. Viscosity radius in dilute polymer solutions: Universal behaviour from DNA rheology and Brownian dynamics simulations. *Macromolecules*, 47(21): 7548–7560, 2014.

[7] C. C. Hua and M. S. Wu. Viscometric properties of dilute polystyrene/dioctyl phthalate solutions. *J. Polym. Sci. Part B Polym. Phys*, 44(5):787–794, 2006.

[8] K.J. Howe, J.C. Crittenden, D.W. Hand, R.R. Trussell, and G. Tchobanoglous. *Principles of Water Treatment.* Wiley, 2012. ISBN 9780470405383. URL `https://books.google.com.au/books?id=igH0BWsYfb0C`.

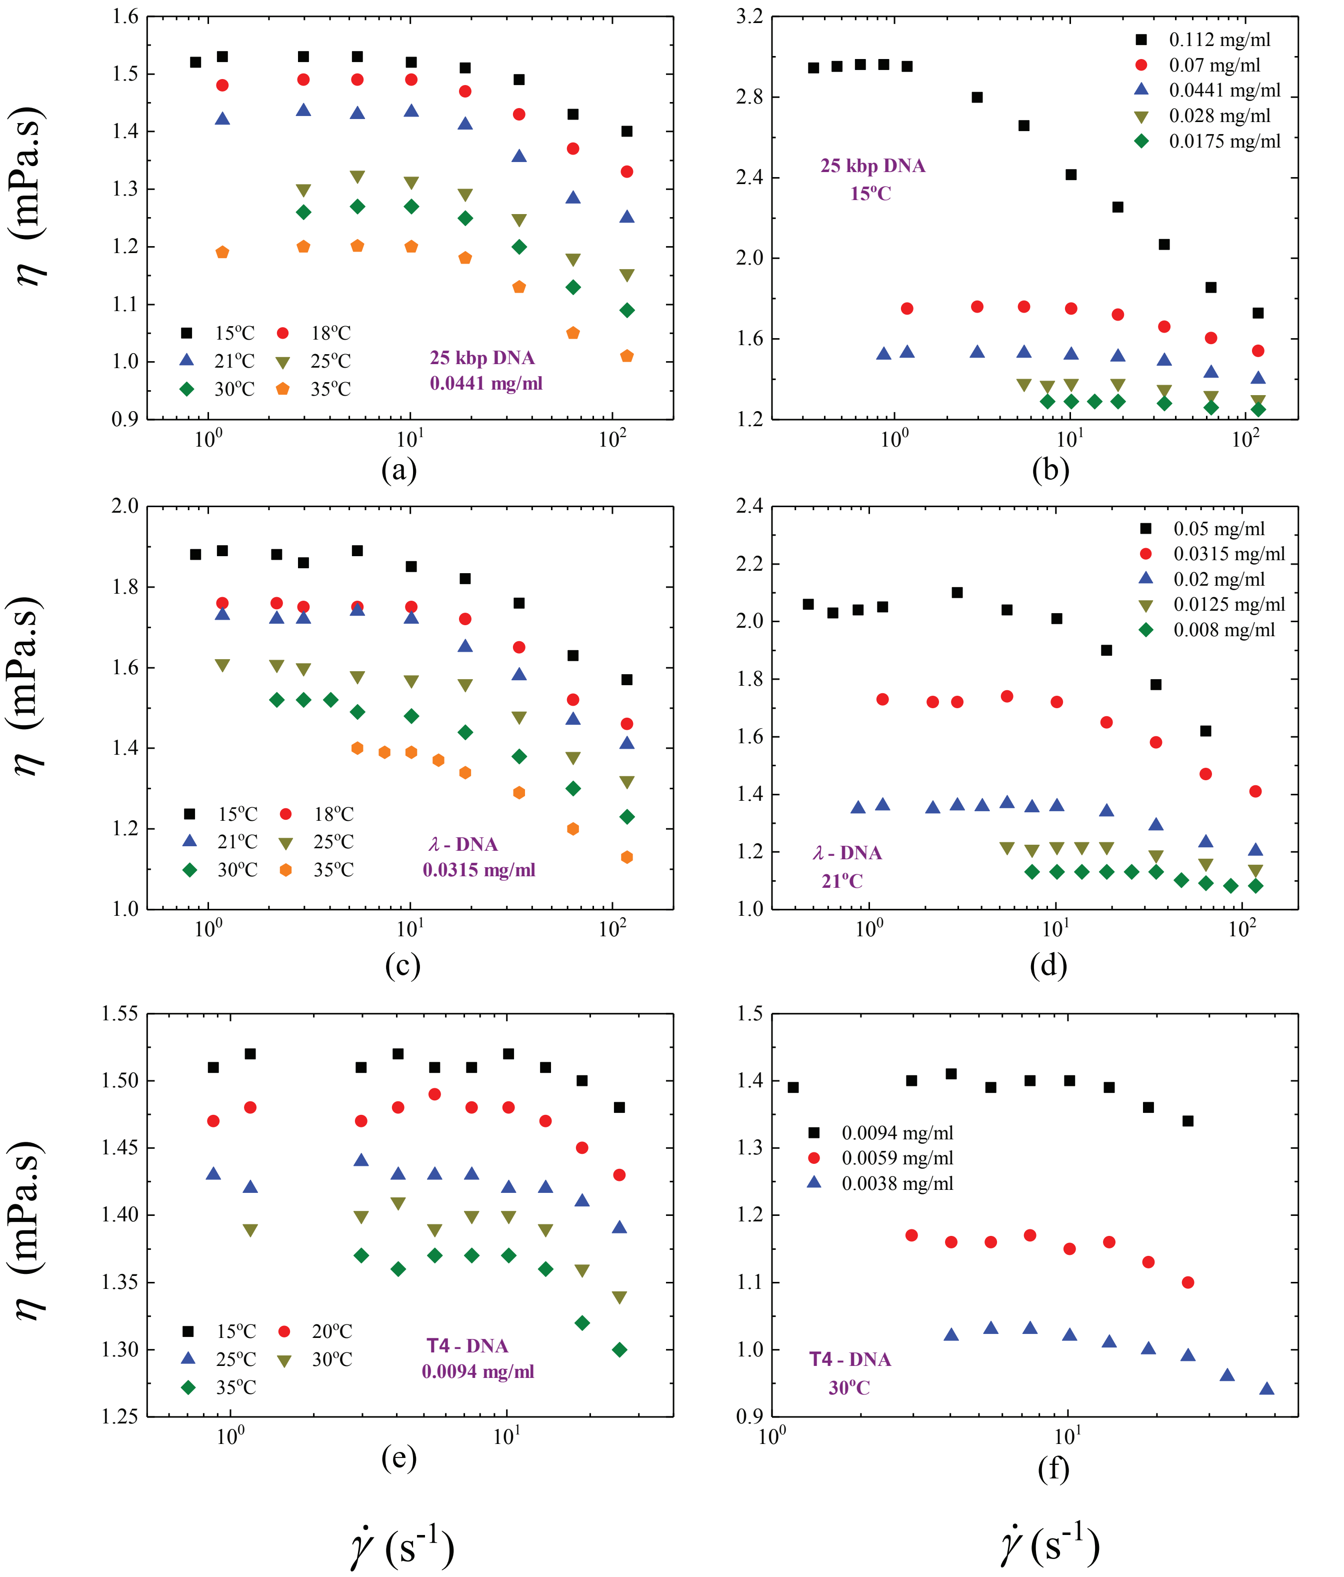


FIG. 3. Shear rate dependence of the viscosity of dilute solutions of 25 kbp, $\lambda$-phage, and T4 DNA. (a), (c) and (e) display dependence at fixed concentrations and various temperatures, while (b), (d) and (f) display dependence at fixed temperatures and various concentrations.

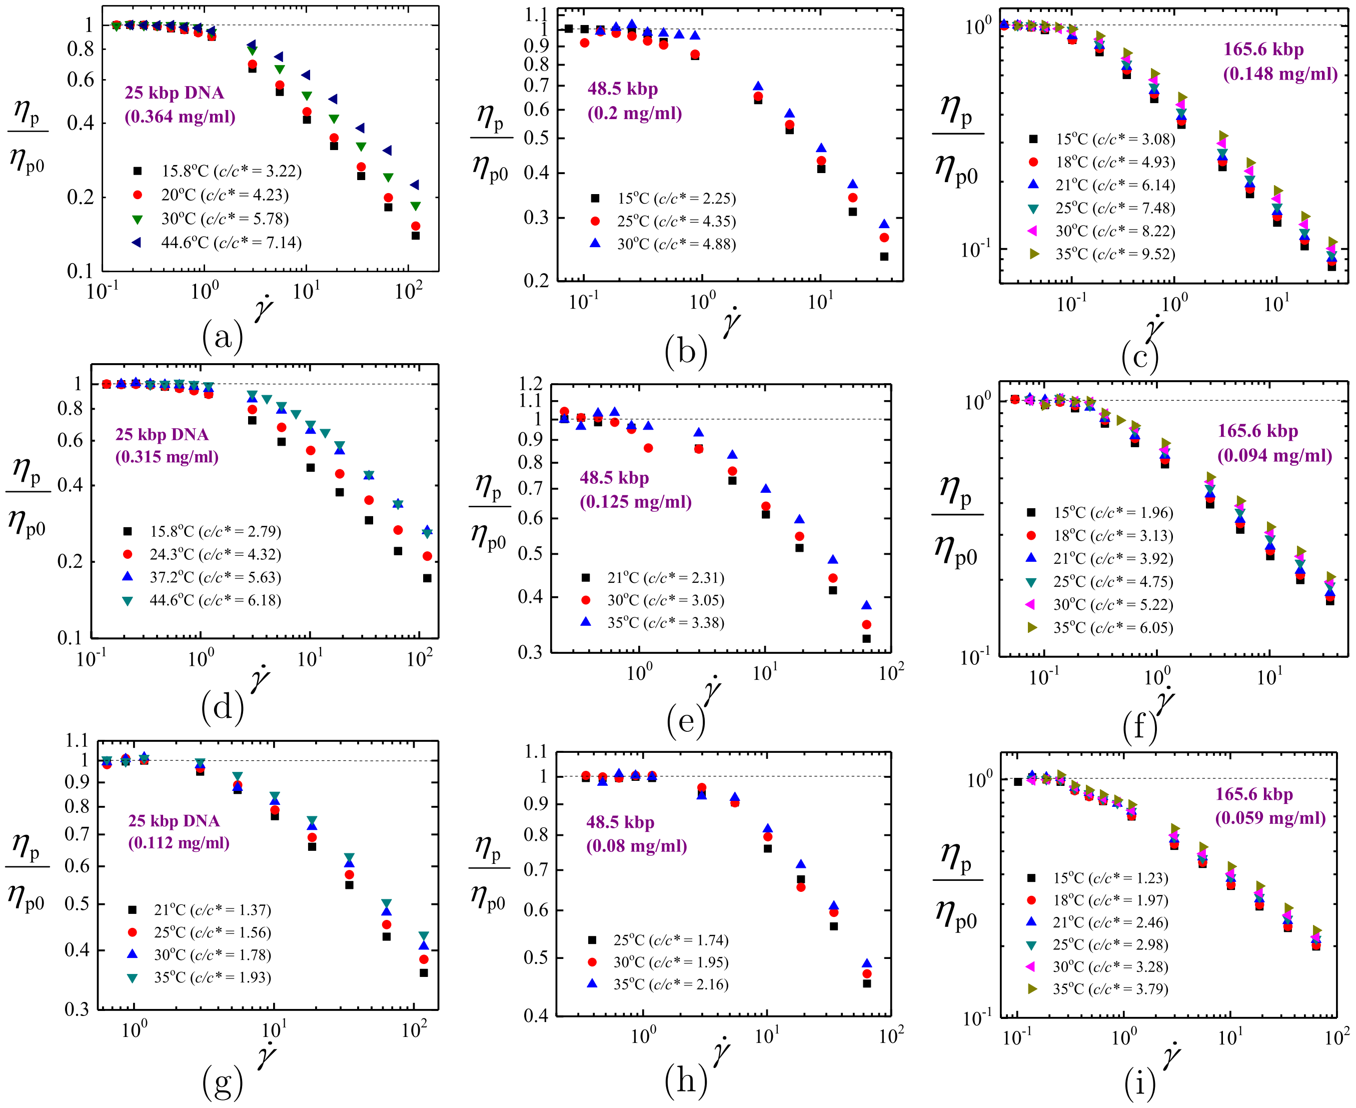


FIG. 4. The ratio $\eta_p/\eta_{p0}$ as a function of shear rate $\dot{\gamma}$, for semidilute solutions of 25 kbp, 48.5 kbp DNA and T4 DNA, each at a fixed absolute concentration and at different temperatures. The temperatures are indicated in the legends and the concentrations are mentioned in individual figures. The values of $\eta_0$ corresponding to the various $c/c^*$ are listed in Table III.

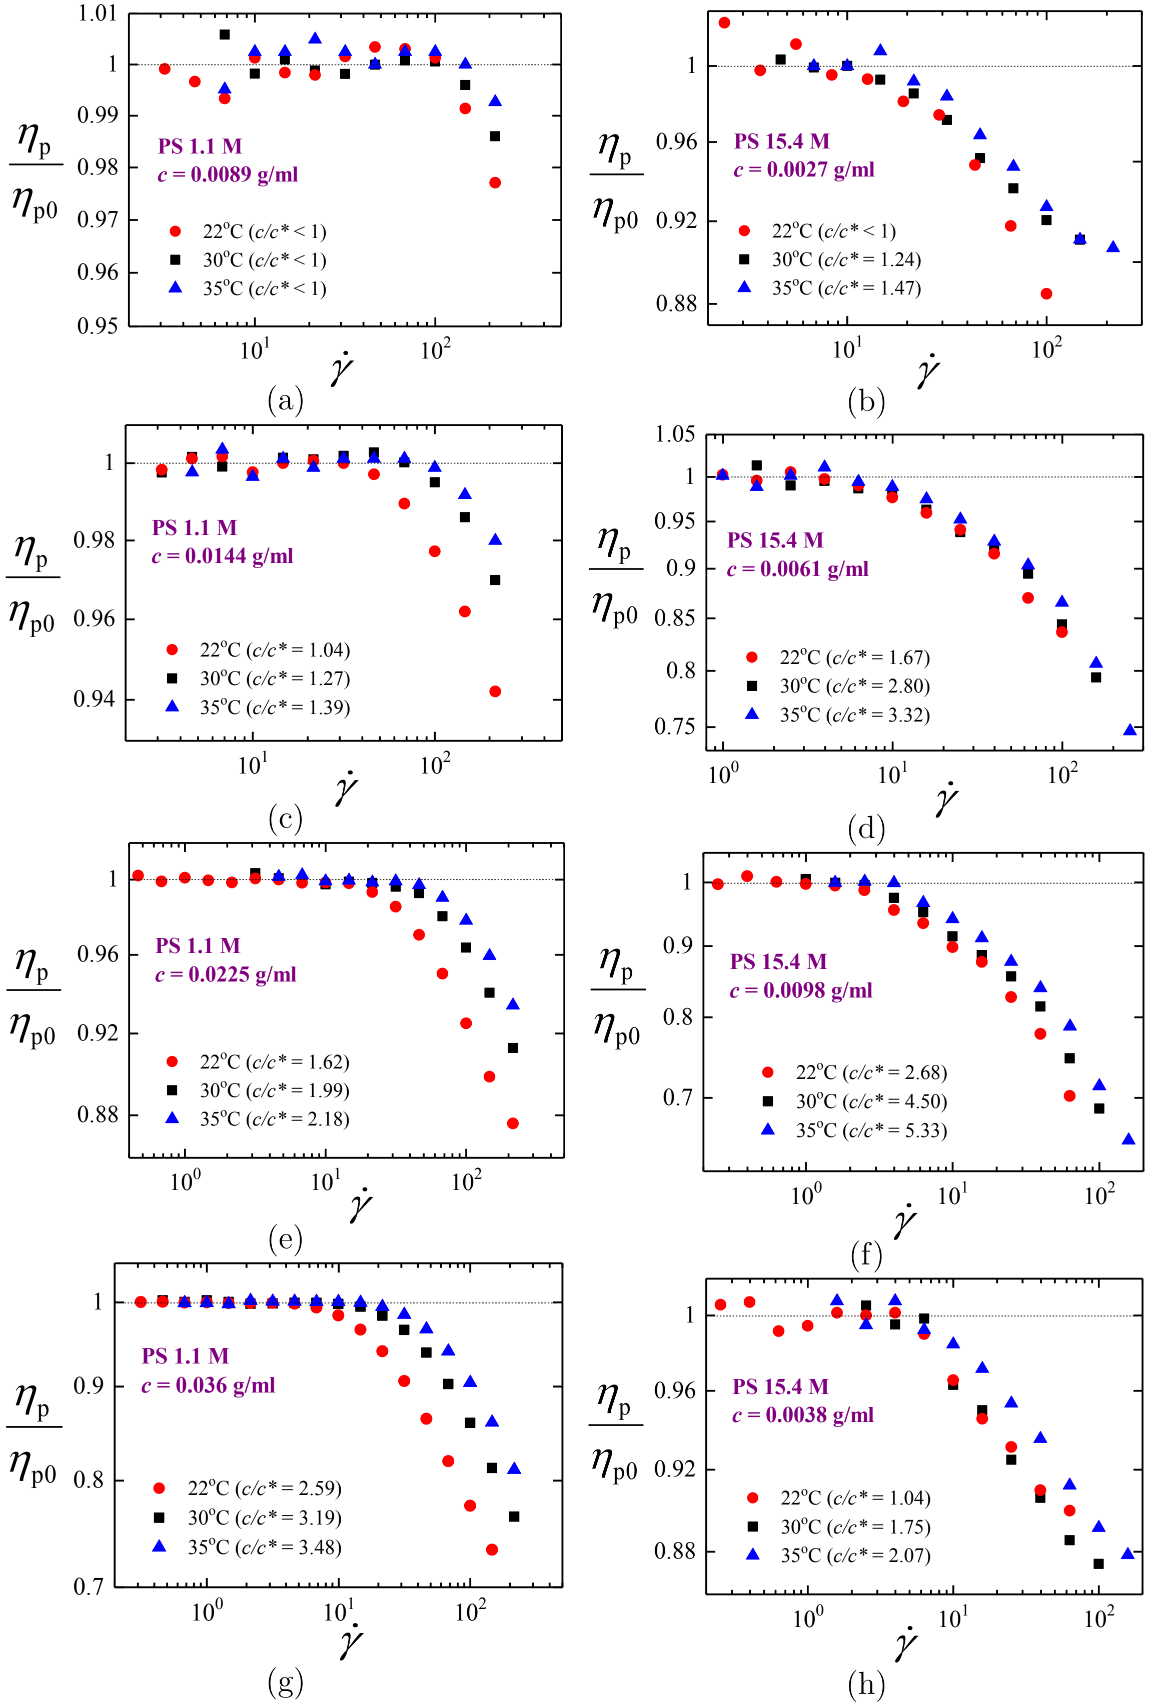


FIG. 5. The ratio $\eta_p/\eta_{p0}$ as a function of shear rate $\dot{\gamma}$, for semidilute solutions of linear 1.1 M and 15.4 M polystyrene samples, each at a fixed absolute concentration and at different temperatures. The temperatures are indicated in the legends and the concentrations are mentioned in individual figures. The values of $\eta_0$ corresponding to the various $c/c^*$ are listed in Table IV.

TABLE V. Data corresponding to the dilute solution shear viscosity $\eta$ (in mPa.s) as a function of shear rate $\dot{\gamma}$ (in $s^{-1}$) displayed in Figs 3 (a) and (b) for dilute 25 kbp DNA samples, at different absolute concentrations $c$ (in mg/ml), and at different temperatures $T$ (in °C). Solvent viscosities $\eta_s$ (in mPa.s) corresponding to different temperatures are also given.

Dilute solution viscosity versus shear rate data for 25 kbp in Figs 3 (a) and (b)

(a) $c = 0.0441$ mg/ml

| $T = 15°C$ | | $T = 18°C$ | | $T = 21°C$ | | $T = 25°C$ | | $T = 30°C$ | | $T = 35°C$ | |
|---|---|---|---|---|---|---|---|---|---|---|---|
| $\eta_s = 1.139$ | | $\eta_s = 1.054$ | | $\eta_s = 0.979$ | | $\eta_s = 0.891$ | | $\eta_s = 0.798$ | | $\eta_s = 0.72$ | |
| $\dot{\gamma}$ | $\eta$ | $\dot{\gamma}$ | $\eta$ | $\dot{\gamma}$ | $\eta$ | $\dot{\gamma}$ | $\eta$ | $\dot{\gamma}$ | $\eta$ | $\dot{\gamma}$ | $\eta$ |
| 0.87 | 1.52 | 1.182 | 1.48 | 1.182 | 1.42 | 2.97 | 1.30 | 2.97 | 1.26 | 1.182 | 1.19 |
| 1.182 | 1.53 | 2.97 | 1.49 | 2.97 | 1.44 | 5.49 | 1.32 | 5.49 | 1.27 | 2.97 | 1.20 |
| 2.97 | 1.53 | 5.49 | 1.49 | 5.49 | 1.43 | 10.15 | 1.31 | 10.15 | 1.27 | 5.49 | 1.20 |
| 5.49 | 1.53 | 10.15 | 1.49 | 10.15 | 1.43 | 18.74 | 1.29 | 18.74 | 1.25 | 10.15 | 1.20 |
| 10.15 | 1.52 | 18.74 | 1.47 | 18.74 | 1.41 | 34.6 | 1.25 | 34.6 | 1.20 | 18.74 | 1.18 |
| 18.74 | 1.51 | 34.6 | 1.43 | 34.6 | 1.36 | 63.9 | 1.18 | 63.9 | 1.13 | 34.6 | 1.13 |
| 34.6 | 1.49 | 63.9 | 1.37 | 63.9 | 1.28 | 118.2 | 1.15 | 118.2 | 1.09 | 63.9 | 1.05 |
| 63.9 | 1.43 | 118.2 | 1.33 | 118.2 | 1.25 | | | | | 118.2 | 1.01 |
| 118.2 | 1.40 | | | | | | | | | | |

(b) $T = 15°C$; $\eta_s = 1.139$ mPa.s

| $c = 0.112$ mg/ml | | $c = 0.07$ mg/ml | | $c = 0.0441$ mg/ml | | $c = 0.028$ mg/ml | | $c = 0.0175$ mg/ml | |
|---|---|---|---|---|---|---|---|---|---|
| $\dot{\gamma}$ | $\eta$ | $\dot{\gamma}$ | $\eta$ | $\dot{\gamma}$ | $\eta$ | $\dot{\gamma}$ | $\eta$ | $\dot{\gamma}$ | $\eta$ |
| 0.346 | 2.94 | 1.182 | 1.75 | 0.87 | 1.52 | 5.49 | 1.38 | 7.46 | 1.29 |
| 0.471 | 2.95 | 2.97 | 1.76 | 1.182 | 1.53 | 7.46 | 1.37 | 10.15 | 1.29 |
| 0.639 | 2.96 | 5.49 | 1.76 | 2.97 | 1.53 | 10.15 | 1.38 | 13.79 | 1.29 |
| 0.87 | 2.96 | 10.15 | 1.75 | 5.49 | 1.53 | 18.74 | 1.38 | 18.74 | 1.29 |
| 1.182 | 2.95 | 18.74 | 1.72 | 10.15 | 1.52 | 34.6 | 1.35 | 34.6 | 1.28 |
| 2.97 | 2.80 | 34.6 | 1.66 | 18.74 | 1.51 | 63.9 | 1.32 | 63.9 | 1.26 |
| 5.49 | 2.66 | 63.9 | 1.61 | 34.6 | 1.49 | 118.2 | 1.30 | 118.2 | 1.25 |
| 10.15 | 2.41 | 118.2 | 1.54 | 63.9 | 1.43 | | | | |
| 18.74 | 2.25 | | | 118.2 | 1.40 | | | | |
| 34.6 | 2.07 | | | | | | | | |
| 63.9 | 1.86 | | | | | | | | |
| 118.2 | 1.73 | | | | | | | | |

TABLE VI. Data corresponding to the dilute solution shear viscosity $\eta$ (in mPa.s) as a function of shear rate $\dot{\gamma}$ (in $s^{-1}$) displayed in Figs 3 (c) and (d) for dilute 48.5 kbp DNA samples at different absolute concentrations $c$ (in mg/ml) and at different temperatures $T$ (in °C). Solvent viscosities $\eta_s$ (in mPa.s) corresponding to different temperatures are also given.

Dilute solution viscosity versus shear rate data for 48.5 kbp in Figs 3 (c) and (d)

(c) $c = 0.0315$ mg/ml

| $T = 15$°C | | $T = 18$°C | | $T = 21$°C | | $T = 25$°C | | $T = 30$°C | | $T = 35$°C | |
|---|---|---|---|---|---|---|---|---|---|---|---|
| $\eta_s = 1.139$ | | $\eta_s = 1.054$ | | $\eta_s = 0.979$ | | $\eta_s = 0.891$ | | $\eta_s = 0.798$ | | $\eta_s = 0.72$ | |
| $\dot{\gamma}$ | $\eta$ | $\dot{\gamma}$ | $\eta$ | $\dot{\gamma}$ | $\eta$ | $\dot{\gamma}$ | $\eta$ | $\dot{\gamma}$ | $\eta$ | $\dot{\gamma}$ | $\eta$ |
| 0.87 | 1.88 | 1.182 | 1.76 | 1.182 | 1.73 | 1.182 | 1.61 | 2.19 | 1.52 | 5.49 | 1.40 |
| 1.182 | 1.89 | 2.19 | 1.76 | 2.19 | 1.72 | 2.19 | 1.61 | 2.97 | 1.52 | 7.46 | 1.39 |
| 2.19 | 1.88 | 2.97 | 1.75 | 2.97 | 1.72 | 2.97 | 1.60 | 4.04 | 1.52 | 10.15 | 1.39 |
| 2.97 | 1.86 | 5.49 | 1.75 | 5.49 | 1.74 | 5.49 | 1.58 | 5.49 | 1.49 | 13.79 | 1.37 |
| 5.49 | 1.89 | 10.15 | 1.75 | 10.15 | 1.72 | 10.15 | 1.57 | 10.15 | 1.48 | 18.74 | 1.34 |
| 10.15 | 1.85 | 18.74 | 1.72 | 18.74 | 1.65 | 18.74 | 1.56 | 18.74 | 1.44 | 34.6 | 1.29 |
| 18.74 | 1.82 | 34.6 | 1.65 | 34.6 | 1.58 | 34.6 | 1.48 | 34.6 | 1.38 | 63.9 | 1.20 |
| 34.6 | 1.76 | 63.9 | 1.52 | 63.9 | 1.47 | 63.9 | 1.38 | 63.9 | 1.30 | 118.2 | 1.13 |
| 63.9 | 1.63 | 118.2 | 1.46 | 118.2 | 1.41 | 118.2 | 1.32 | 118.2 | 1.23 | | |
| 118.2 | 1.57 | | | | | | | | | | |

(d) $T = 21$°C; $\eta_s = 0.979$ mPa.s

| $c = 0.05$ mg/ml | | $c = 0.0315$ mg/ml | | $c = 0.02$ mg/ml | | $c = 0.0125$ mg/ml | | $c = 0.008$ mg/ml | |
|---|---|---|---|---|---|---|---|---|---|
| $\dot{\gamma}$ | $\eta$ | $\dot{\gamma}$ | $\eta$ | $\dot{\gamma}$ | $\eta$ | $\dot{\gamma}$ | $\eta$ | $\dot{\gamma}$ | $\eta$ |
| 0.471 | 2.06 | 1.182 | 1.73 | 0.87 | 1.35 | 5.49 | 1.22 | 7.46 | 1.13 |
| 0.639 | 2.03 | 2.19 | 1.72 | 1.182 | 1.36 | 7.46 | 1.21 | 10.15 | 1.13 |
| 0.87 | 2.04 | 2.97 | 1.72 | 2.19 | 1.35 | 10.15 | 1.22 | 13.79 | 1.13 |
| 1.182 | 2.05 | 5.49 | 1.74 | 2.97 | 1.36 | 13.79 | 1.22 | 18.74 | 1.13 |
| 2.97 | 2.10 | 10.15 | 1.72 | 4.04 | 1.36 | 18.74 | 1.22 | 25.5 | 1.13 |
| 5.49 | 2.04 | 18.74 | 1.65 | 5.49 | 1.37 | 34.6 | 1.19 | 34.6 | 1.13 |
| 10.15 | 2.01 | 34.6 | 1.58 | 7.46 | 1.35 | 63.9 | 1.16 | 47.1 | 1.10 |
| 18.74 | 1.90 | 63.9 | 1.47 | 10.15 | 1.36 | 118.2 | 1.14 | 63.9 | 1.09 |
| 34.6 | 1.78 | 118.2 | 1.41 | 18.74 | 1.34 | | | 87 | 1.08 |
| 63.9 | 1.62 | | | 34.6 | 1.29 | | | 118.2 | 1.08 |
| | | | | 63.9 | 1.23 | | | | |
| | | | | 118.2 | 1.20 | | | | |

TABLE VII. Data corresponding to the dilute solution shear viscosity $\eta$ (in mPa.s) as a function of shear rate $\dot{\gamma}$ (in $s^{-1}$) displayed in Figs 3 (e) and (f) for dilute 165.6 kbp DNA samples at different absolute concentrations $c$ (in mg/ml) and at different temperatures $T$ (in °C). Solvent viscosities $\eta_s$ (in mPa.s) corresponding to different temperatures are also given.

Dilute solution viscosity versus shear rate data for 165.6 kbp in Figs 3 (e) and (f)

(e) $c = 0.0094$ mg/ml

| $T = 15°C$ | | $T = 20°C$ | | $T = 25°C$ | | $T = 30°C$ | | $T = 35°C$ | |
|---|---|---|---|---|---|---|---|---|---|
| $\eta_s = 1.139$ | | $\eta_s = 1.01$ | | $\eta_s = 0.891$ | | $\eta_s = 0.798$ | | $\eta_s = 0.72$ | |
| $\dot{\gamma}$ | $\eta$ | $\dot{\gamma}$ | $\eta$ | $\dot{\gamma}$ | $\eta$ | $\dot{\gamma}$ | $\eta$ | $\dot{\gamma}$ | $\eta$ |
| 0.87 | 1.51 | 0.87 | 1.47 | 0.87 | 1.43 | 1.182 | 1.39 | 2.97 | 1.37 |
| 1.182 | 1.52 | 1.182 | 1.48 | 1.182 | 1.42 | 2.97 | 1.40 | 4.04 | 1.36 |
| 2.97 | 1.51 | 2.97 | 1.47 | 2.97 | 1.44 | 4.04 | 1.41 | 5.49 | 1.37 |
| 4.04 | 1.52 | 4.04 | 1.48 | 4.04 | 1.43 | 5.49 | 1.39 | 7.46 | 1.37 |
| 5.49 | 1.51 | 5.49 | 1.49 | 5.49 | 1.43 | 7.46 | 1.40 | 10.15 | 1.37 |
| 7.46 | 1.51 | 7.46 | 1.48 | 7.46 | 1.43 | 10.15 | 1.40 | 13.79 | 1.36 |
| 10.15 | 1.52 | 10.15 | 1.48 | 10.15 | 1.42 | 13.79 | 1.39 | 18.74 | 1.32 |
| 13.79 | 1.51 | 13.79 | 1.47 | 13.79 | 1.42 | 18.74 | 1.36 | 25.5 | 1.30 |
| 18.74 | 1.50 | 18.74 | 1.45 | 18.74 | 1.41 | 25.5 | 1.34 | | |
| 25.5 | 1.48 | 25.5 | 1.43 | 25.5 | 1.39 | | | | |

(f) $T = 30°C$; $\eta_s = 0.798$ mPa.s

| $c = 0.0094$ mg/ml | | $c = 0.0059$ mg/ml | | $c = 0.0038$ mg/ml | |
|---|---|---|---|---|---|
| $\dot{\gamma}$ | $\eta$ | $\dot{\gamma}$ | $\eta$ | $\dot{\gamma}$ | $\eta$ |
| 1.182 | 1.39 | 2.97 | 1.17 | 4.04 | 1.02 |
| 2.97 | 1.40 | 4.04 | 1.16 | 5.49 | 1.03 |
| 4.04 | 1.41 | 5.49 | 1.16 | 7.46 | 1.03 |
| 5.49 | 1.39 | 7.46 | 1.17 | 10.15 | 1.02 |
| 7.46 | 1.40 | 10.15 | 1.15 | 13.79 | 1.01 |
| 10.15 | 1.40 | 13.79 | 1.16 | 18.74 | 1.00 |
| 13.79 | 1.39 | 18.74 | 1.13 | 25.5 | 0.99 |
| 18.74 | 1.36 | 25.5 | 1.10 | 34.6 | 0.96 |
| 25.5 | 1.34 | | | 47.1 | 0.94 |

TABLE VIII. Data corresponding to the semidilute solution shear viscosity $\eta$ (in mPa.s) as a function of shear rate $\dot{\gamma}$ (in $s^{-1}$) displayed in Figs 4 (a) and (b) for DNA samples at different absolute concentrations $c$ (in mg/ml) and at different temperatures $T$ (in °C). Solvent viscosities $\eta_s$ (in mPa.s) corresponding to different temperatures are also given.

| | 25 kbp | | | | | | | |
|---|---|---|---|---|---|---|---|---|
| | $c = 0.364$ mg/ml | | | | | | | |
| | $T = 15.8$°C | | $T = 20$°C | | $T = 30$°C | | $T = 44.6$°C | |
| (a) | $\eta_s = 1.118$ | | $\eta_s = 1.01$ | | $\eta_s = 0.798$ | | $\eta_s = 0.6$ | |
| | $\dot{\gamma}$ | $\eta$ | $\dot{\gamma}$ | $\eta$ | $\dot{\gamma}$ | $\eta$ | $\dot{\gamma}$ | $\eta$ |
| | 0.1379 | 20.4 | 0.1379 | 17.8 | 0.1379 | 12.7 | 0.1874 | 8.6 |
| | 0.1874 | 20.5 | 0.1874 | 17.8 | 0.1874 | 12.9 | 0.255 | 8.5 |
| | 0.255 | 20.4 | 0.255 | 17.8 | 0.255 | 12.8 | 0.346 | 8.5 |
| | 0.346 | 20.2 | 0.346 | 17.6 | 0.346 | 12.8 | 0.471 | 8.5 |
| | 0.471 | 19.8 | 0.471 | 17.3 | 0.471 | 12.8 | 0.639 | 8.4 |
| | 0.639 | 19.6 | 0.639 | 17.1 | 0.639 | 12.8 | 0.87 | 8.3 |
| | 0.87 | 19.2 | 0.87 | 16.6 | 0.87 | 12.5 | 1.182 | 8.1 |
| | 1.182 | 18.4 | 1.182 | 16.1 | 1.182 | 12.0 | 2.97 | 7.2 |
| | 2.97 | 14.0 | 2.97 | 12.6 | 2.97 | 10.3 | 5.49 | 6.5 |
| | 5.49 | 11.5 | 5.49 | 10.6 | 5.49 | 8.8 | 10.15 | 5.6 |
| | 10.15 | 9.1 | 10.15 | 8.5 | 10.15 | 7.1 | 18.74 | 4.6 |
| | 18.74 | 7.4 | 18.74 | 6.9 | 18.74 | 5.9 | 34.6 | 3.6 |
| | 34.6 | 5.9 | 34.6 | 5.5 | 34.6 | 4.7 | 63.9 | 3.1 |
| | 63.9 | 4.7 | 63.9 | 4.4 | 63.9 | 3.8 | 118.2 | 2.4 |
| | 118.2 | 3.9 | 118.2 | 3.6 | 118.2 | 3.1 | | |

| | λ-DNA, 48.5 kbp | | | | | |
|---|---|---|---|---|---|---|
| | $c = 0.2$ mg/ml | | | | | |
| | $T = 15$°C | | $T = 25$°C | | $T = 30$°C | |
| (b) | $\eta_s = 1.139$ | | $\eta_s = 0.891$ | | $\eta_s = 0.798$ | |
| | $\dot{\gamma}$ | $\eta$ | $\dot{\gamma}$ | $\eta$ | $\dot{\gamma}$ | $\eta$ |
| | 0.0746 | 16.1 | 0.1015 | 12.1 | 0.1379 | 11.3 |
| | 0.1015 | 16.1 | 0.1379 | 13.0 | 0.1874 | 11.6 |
| | 0.1379 | 16.1 | 0.1874 | 12.9 | 0.255 | 11.8 |
| | 0.1874 | 15.9 | 0.255 | 12.6 | 0.346 | 11.2 |
| | 0.255 | 16.0 | 0.346 | 12.3 | 0.471 | 11.2 |
| | 0.346 | 15.6 | 0.471 | 12.0 | 0.639 | 11.1 |
| | 0.471 | 14.9 | 0.87 | 11.3 | 0.87 | 11.0 |
| | 0.87 | 13.7 | 2.97 | 8.9 | 2.97 | 8.2 |
| | 2.97 | 10.6 | 5.49 | 7.6 | 5.49 | 7.0 |
| | 5.49 | 9.0 | 10.15 | 6.2 | 10.15 | 5.8 |
| | 10.15 | 7.2 | 18.74 | 5.1 | 18.74 | 4.7 |
| | 18.74 | 5.8 | 34.6 | 4.1 | 34.6 | 3.8 |
| | 34.6 | 4.6 | | | | |

TABLE IX. Data corresponding to the semidilute solution shear viscosity $\eta$ (in mPa.s) as a function of shear rate $\dot{\gamma}$ (in $s^{-1}$) displayed in Figs 4 (c) and (d) for DNA samples at different absolute concentrations $c$ (in mg/ml) and at different temperatures $T$ (in °C). Solvent viscosities $\eta_s$ (in mPa.s) corresponding to different temperatures are also given.

| T4 DNA, 165.6 kbp | | | | | | | | | | | | |
|---|---|---|---|---|---|---|---|---|---|---|---|---|
| | $c = 0.148$ mg/ml | | | | | | | | | | | |
| | $T = 15°C$ | | $T = 18°C$ | | $T = 21°C$ | | $T = 25°C$ | | $T = 30°C$ | | $T = 35°C$ | |
| (c) | $\eta_s = 1.139$ | | $\eta_s = 1.054$ | | $\eta_s = 0.979$ | | $\eta_s = 0.891$ | | $\eta_s = 0.798$ | | $\eta_s = 0.72$ | |
| | $\dot{\gamma}$ | $\eta$ | $\dot{\gamma}$ | $\eta$ | $\dot{\gamma}$ | $\eta$ | $\dot{\gamma}$ | $\eta$ | $\dot{\gamma}$ | $\eta$ | $\dot{\gamma}$ | $\eta$ |
| | 0.0219 | 56.5 | 0.0219 | 50.8 | 0.0219 | 47.3 | 0.0297 | 42.8 | 0.0297 | 37.3 | 0.0297 | 32.5 |
| | 0.0297 | 56.1 | 0.0297 | 51.1 | 0.0297 | 47.0 | 0.0404 | 42.7 | 0.0404 | 37.1 | 0.0404 | 32.7 |
| | 0.0404 | 55.2 | 0.0404 | 50.2 | 0.0404 | 46.5 | 0.0549 | 42.1 | 0.0549 | 36.8 | 0.0549 | 32.6 |
| | 0.0549 | 53.7 | 0.0549 | 49.5 | 0.0549 | 46.1 | 0.1015 | 40.8 | 0.0746 | 36.1 | 0.0746 | 32.0 |
| | 0.1015 | 48.6 | 0.1015 | 44.1 | 0.1015 | 42.2 | 0.1874 | 35.4 | 0.1015 | 35.2 | 0.1015 | 31.4 |
| | 0.1874 | 42.9 | 0.1874 | 40.5 | 0.1874 | 38.3 | 0.346 | 29.0 | 0.1874 | 32.5 | 0.1874 | 29.3 |
| | 0.346 | 34.2 | 0.346 | 32.6 | 0.346 | 31.0 | 0.639 | 23.1 | 0.346 | 26.8 | 0.346 | 24.7 |
| | 0.639 | 26.9 | 0.639 | 25.7 | 0.639 | 24.4 | 1.182 | 18.0 | 0.639 | 21.6 | 0.639 | 20.1 |
| | 1.182 | 20.9 | 1.182 | 19.7 | 1.182 | 18.9 | 2.97 | 12.2 | 1.182 | 16.9 | 1.182 | 15.9 |
| | 2.97 | 13.9 | 2.97 | 13.3 | 2.97 | 12.8 | 5.49 | 9.5 | 2.97 | 11.6 | 2.97 | 10.9 |
| | 5.49 | 10.8 | 5.49 | 10.3 | 5.49 | 9.9 | 10.15 | 7.3 | 5.49 | 8.9 | 5.49 | 8.4 |
| | 10.15 | 8.3 | 10.15 | 8.0 | 10.15 | 7.7 | 18.74 | 5.8 | 10.15 | 6.9 | 10.15 | 6.5 |
| | 18.74 | 6.8 | 18.74 | 6.5 | 18.74 | 6.2 | 34.6 | 4.8 | 18.74 | 5.5 | 18.74 | 5.2 |
| | 34.6 | 5.7 | 34.6 | 5.4 | 34.6 | 5.1 | | | 34.6 | 4.4 | 34.6 | 4.1 |

| 25 kbp | | | | | | | | |
|---|---|---|---|---|---|---|---|---|
| | $c = 0.315$ mg/ml | | | | | | | |
| | $T = 15.8°C$ | | $T = 24.3°C$ | | $T = 37.2°C$ | | $T = 44.6°C$ | |
| (d) | $\eta_s = 1.118$ | | $\eta_s = 0.905$ | | $\eta_s = 0.689$ | | $\eta_s = 0.6$ | |
| | $\dot{\gamma}$ | $\eta$ | $\dot{\gamma}$ | $\eta$ | $\dot{\gamma}$ | $\eta$ | $\dot{\gamma}$ | $\eta$ |
| | 0.1379 | 14.7 | 0.1379 | 11.2 | 0.1874 | 7.7 | 0.346 | 6.6 |
| | 0.1874 | 14.7 | 0.1874 | 11.1 | 0.255 | 7.7 | 0.471 | 6.6 |
| | 0.255 | 14.8 | 0.255 | 11.2 | 0.346 | 7.7 | 0.639 | 6.7 |
| | 0.346 | 14.7 | 0.346 | 11.1 | 0.471 | 7.6 | 0.87 | 6.6 |
| | 0.471 | 14.4 | 0.471 | 11.0 | 0.639 | 7.6 | 1.182 | 6.5 |
| | 0.639 | 14.3 | 0.639 | 10.8 | 0.87 | 7.5 | 2.97 | 6.1 |
| | 0.87 | 14.1 | 0.87 | 10.6 | 1.182 | 7.4 | 4.04 | 5.9 |
| | 1.182 | 13.6 | 1.182 | 10.3 | 2.97 | 6.8 | 5.49 | 5.6 |
| | 2.97 | 10.9 | 2.97 | 9.1 | 5.49 | 6.2 | 7.46 | 5.2 |
| | 5.49 | 9.2 | 5.49 | 7.8 | 10.15 | 5.3 | 10.15 | 4.8 |
| | 10.15 | 7.5 | 10.15 | 6.5 | 18.74 | 4.5 | 13.79 | 4.5 |
| | 18.74 | 6.3 | 18.74 | 5.5 | 34.6 | 3.7 | 18.74 | 4.1 |
| | 34.6 | 5.1 | 34.6 | 4.5 | 63.9 | 3.0 | 34.6 | 3.3 |
| | 63.9 | 4.2 | 63.9 | 3.6 | 118.2 | 2.5 | 63.9 | 2.6 |
| | 118.2 | 3.5 | 118.2 | 3.1 | | | 118.2 | 2.2 |

TABLE X. Data corresponding to the semidilute solution shear viscosity $\eta$ (in mPa.s) as a function of shear rate $\dot{\gamma}$ (in $s^{-1}$) displayed in Figs 4 (e) and (f) for DNA samples at different absolute concentrations $c$ (in mg/ml) and at different temperatures $T$ (in °C). Solvent viscosities $\eta_s$ (in mPa.s) corresponding to different temperatures are also given.

| λ-DNA, 48.5 kbp | | | | | | |
|---|---|---|---|---|---|---|
| | $c = 0.125$ mg/ml | | | | | |
| | $T = 21$°C | | $T = 30$°C | | $T = 35$°C | |
| (e) | $\eta_s = 0.979$ | | $\eta_s = 0.798$ | | $\eta_s = 0.72$ | |
| | $\dot{\gamma}$ | $\eta$ | $\dot{\gamma}$ | $\eta$ | $\dot{\gamma}$ | $\eta$ |
| | 0.255 | 6.1 | 0.255 | 5.2 | 0.255 | 4.4 |
| | 0.346 | 6.2 | 0.346 | 5.1 | 0.346 | 4.2 |
| | 0.471 | 6.1 | 0.471 | 5.1 | 0.471 | 4.5 |
| | 0.87 | 5.9 | 0.639 | 5.0 | 0.639 | 4.5 |
| | 2.97 | 5.4 | 0.87 | 4.8 | 0.87 | 4.3 |
| | 5.49 | 4.7 | 1.182 | 4.5 | 1.182 | 4.2 |
| | 10.15 | 4.1 | 2.97 | 4.4 | 2.97 | 4.1 |
| | 18.74 | 3.6 | 5.49 | 4.1 | 5.49 | 3.8 |
| | 34.6 | 3.1 | 10.15 | 3.5 | 10.15 | 3.3 |
| | 63.9 | 2.6 | 18.74 | 3.1 | 18.74 | 2.9 |
| | | | 34.6 | 2.7 | 34.6 | 2.5 |
| | | | 63.9 | 2.3 | 63.9 | 2.1 |

| T4 DNA, 165.6 kbp | | | | | | | | | | | | |
|---|---|---|---|---|---|---|---|---|---|---|---|---|
| | $c = 0.094$ mg/ml | | | | | | | | | | | |
| | $T = 15$°C | | $T = 18$°C | | $T = 21$°C | | $T = 25$°C | | $T = 30$°C | | $T = 35$°C | |
| (f) | $\eta_s = 1.139$ | | $\eta_s = 1.054$ | | $\eta_s = 0.979$ | | $\eta_s = 0.891$ | | $\eta_s = 0.798$ | | $\eta_s = 0.72$ | |
| | $\dot{\gamma}$ | $\eta$ | $\dot{\gamma}$ | $\eta$ | $\dot{\gamma}$ | $\eta$ | $\dot{\gamma}$ | $\eta$ | $\dot{\gamma}$ | $\eta$ | $\dot{\gamma}$ | $\eta$ |
| | 0.0549 | 19.8 | 0.0549 | 18.0 | 0.0746 | 16.7 | 0.0746 | 14.7 | 0.0746 | 13.0 | 0.1015 | 11.2 |
| | 0.0746 | 19.6 | 0.0746 | 18.0 | 0.1015 | 16.5 | 0.1015 | 14.3 | 0.1015 | 12.7 | 0.1379 | 11.8 |
| | 0.1015 | 18.8 | 0.1015 | 17.3 | 0.1379 | 16.6 | 0.1379 | 14.9 | 0.1379 | 13.2 | 0.1874 | 11.6 |
| | 0.1379 | 19.4 | 0.1379 | 17.6 | 0.1874 | 16.0 | 0.1874 | 14.5 | 0.1874 | 12.9 | 0.255 | 11.6 |
| | 0.1874 | 18.3 | 0.1874 | 17.1 | 0.255 | 15.5 | 0.255 | 14.0 | 0.255 | 12.8 | 0.346 | 10.5 |
| | 0.346 | 16.1 | 0.346 | 15.1 | 0.346 | 14.1 | 0.346 | 12.8 | 0.346 | 11.6 | 0.471 | 9.9 |
| | 0.639 | 13.7 | 0.639 | 13.0 | 0.639 | 12.2 | 0.639 | 11.3 | 0.639 | 10.3 | 0.639 | 9.5 |
| | 1.182 | 11.5 | 1.182 | 10.9 | 1.182 | 10.4 | 1.182 | 9.5 | 1.182 | 8.6 | 1.182 | 8.2 |
| | 2.97 | 8.4 | 2.97 | 8.0 | 2.97 | 7.6 | 2.97 | 7.1 | 2.97 | 6.7 | 2.97 | 6.2 |
| | 5.49 | 6.9 | 5.49 | 6.6 | 5.49 | 6.3 | 5.49 | 5.9 | 5.49 | 5.5 | 5.49 | 5.2 |
| | 10.15 | 5.7 | 10.15 | 5.4 | 10.15 | 5.1 | 10.15 | 4.8 | 10.15 | 4.5 | 10.15 | 4.2 |
| | 18.74 | 4.8 | 18.74 | 4.5 | 18.74 | 4.3 | 18.74 | 4.1 | 18.74 | 3.8 | 18.74 | 3.5 |
| | 34.6 | 4.2 | 34.6 | 3.9 | 34.6 | 3.7 | 34.6 | 3.5 | 34.6 | 3.2 | 34.6 | 3.0 |

TABLE XI. Data corresponding to the semidilute solution shear viscosity $\eta$ (in mPa.s) as a function of shear rate $\dot{\gamma}$ (in $s^{-1}$) displayed in Figs 4 (g), (h) and (i) for DNA samples at different absolute concentrations $c$ (in mg/ml) and at different temperatures $T$ (in °C). Solvent viscosities $\eta_s$ (in mPa.s) corresponding to different temperatures are also given.

| 25 kbp | | | | | | | | |
|---|---|---|---|---|---|---|---|---|
| | $c = 0.112$ mg/ml | | | | | | | |
| | $T = 21$°C | | $T = 25$°C | | $T = 30$°C | | $T = 35$°C | |
| (g) | $\eta_s = 0.979$ | | $\eta_s = 0.891$ | | $\eta_s = 0.798$ | | $\eta_s = 0.72$ | |
| | $\dot{\gamma}$ | $\eta$ | $\dot{\gamma}$ | $\eta$ | $\dot{\gamma}$ | $\eta$ | $\dot{\gamma}$ | $\eta$ |
| | 0.639 | 2.5 | 0.639 | 2.3 | 0.639 | 2.0 | 0.639 | 1.8 |
| | 0.87 | 2.5 | 0.87 | 2.3 | 0.87 | 2.0 | 0.87 | 1.8 |
| | 1.182 | 2.5 | 1.182 | 2.3 | 1.182 | 2.1 | 1.182 | 1.9 |
| | 2.97 | 2.4 | 2.97 | 2.2 | 2.97 | 2.0 | 2.97 | 1.8 |
| | 5.49 | 2.3 | 5.49 | 2.1 | 5.49 | 1.9 | 5.49 | 1.8 |
| | 10.15 | 2.2 | 10.15 | 2.0 | 10.15 | 1.8 | 10.15 | 1.7 |
| | 18.74 | 2.0 | 18.74 | 1.8 | 18.74 | 1.7 | 18.74 | 1.6 |
| | 34.6 | 1.8 | 34.6 | 1.7 | 34.6 | 1.5 | 34.6 | 1.4 |
| | 63.9 | 1.6 | 63.9 | 1.5 | 63.9 | 1.4 | 63.9 | 1.3 |
| | 118.2 | 1.5 | 118.2 | 1.4 | 118.2 | 1.3 | 118.2 | 1.2 |

| $\lambda$-DNA, 48.5 kbp | | | | | | |
|---|---|---|---|---|---|---|
| | $c = 0.08$ mg/ml | | | | | |
| | $T = 25$°C | | $T = 30$°C | | $T = 35$°C | |
| (h) | $\eta_s = 0.891$ | | $\eta_s = 0.798$ | | $\eta_s = 0.72$ | |
| | $\dot{\gamma}$ | $\eta$ | $\dot{\gamma}$ | $\eta$ | $\dot{\gamma}$ | $\eta$ |
| | 0.346 | 3.1 | 0.346 | 2.8 | 0.471 | 2.5 |
| | 0.471 | 3.1 | 0.471 | 2.8 | 0.639 | 2.6 |
| | 0.639 | 3.1 | 0.639 | 2.8 | 0.87 | 2.5 |
| | 0.87 | 3.1 | 0.87 | 2.8 | 1.182 | 2.5 |
| | 1.182 | 3.1 | 1.182 | 2.8 | 2.97 | 2.4 |
| | 2.97 | 3.0 | 2.97 | 2.7 | 5.49 | 2.4 |
| | 5.49 | 2.9 | 5.49 | 2.6 | 10.15 | 2.2 |
| | 10.15 | 2.6 | 10.15 | 2.4 | 18.74 | 2.0 |
| | 18.74 | 2.4 | 18.74 | 2.1 | 34.6 | 1.8 |
| | 34.6 | 2.2 | 34.6 | 2.0 | 63.9 | 1.6 |
| | 63.9 | 1.9 | 63.9 | 1.7 | | |

| T4 DNA, 165.6 kbp | | | | | | | | | | | | |
|---|---|---|---|---|---|---|---|---|---|---|---|---|
| | $c = 0.059$ mg/ml | | | | | | | | | | | |
| | $T = 15$°C | | $T = 18$°C | | $T = 21$°C | | $T = 25$°C | | $T = 30$°C | | $T = 35$°C | |
| (i) | $\eta_s = 1.139$ | | $\eta_s = 1.054$ | | $\eta_s = 0.979$ | | $\eta_s = 0.891$ | | $\eta_s = 0.798$ | | $\eta_s = 0.72$ | |
| | $\dot{\gamma}$ | $\eta$ | $\dot{\gamma}$ | $\eta$ | $\dot{\gamma}$ | $\eta$ | $\dot{\gamma}$ | $\eta$ | $\dot{\gamma}$ | $\eta$ | $\dot{\gamma}$ | $\eta$ |
| | 0.1015 | 10.0 | 0.1379 | 9.7 | 0.1379 | 9.0 | 0.1379 | 8.1 | 0.1379 | 7.2 | 0.1874 | 6.5 |
| | 0.1379 | 10.4 | 0.1874 | 9.6 | 0.1874 | 8.9 | 0.1874 | 8.1 | 0.1874 | 7.3 | 0.255 | 6.7 |
| | 0.1874 | 10.2 | 0.255 | 9.5 | 0.255 | 8.8 | 0.255 | 8.1 | 0.255 | 7.3 | 0.346 | 6.1 |
| | 0.255 | 10.0 | 0.346 | 8.7 | 0.346 | 8.1 | 0.346 | 7.5 | 0.346 | 6.8 | 0.471 | 5.9 |
| | 0.346 | 9.3 | 0.471 | 8.3 | 0.471 | 7.8 | 0.471 | 7.2 | 0.471 | 6.5 | 0.639 | 5.6 |
| | 0.471 | 8.9 | 0.639 | 8.0 | 0.639 | 7.5 | 0.639 | 6.8 | 0.639 | 6.2 | 0.87 | 5.4 |
| | 0.639 | 8.5 | 1.182 | 7.0 | 0.87 | 7.1 | 0.87 | 6.6 | 0.87 | 6.0 | 1.182 | 5.2 |
| | 1.182 | 7.5 | 2.97 | 5.6 | 1.182 | 6.6 | 1.182 | 6.2 | 1.182 | 5.6 | 2.97 | 4.3 |
| | 2.97 | 5.9 | 5.49 | 4.9 | 2.97 | 5.3 | 2.97 | 5.0 | 2.97 | 4.6 | 5.49 | 3.7 |
| | 5.49 | 5.2 | 10.15 | 4.1 | 5.49 | 4.6 | 5.49 | 4.3 | 5.49 | 4.0 | 10.15 | 3.2 |
| | 10.15 | 4.4 | 18.74 | 3.6 | 10.15 | 3.9 | 10.15 | 3.7 | 10.15 | 3.4 | 18.74 | 2.8 |
| | 18.74 | 3.8 | 34.6 | 3.1 | 18.74 | 3.4 | 18.74 | 3.2 | 18.74 | 3.0 | 34.6 | 2.4 |
| | 34.6 | 3.3 | 63.9 | 2.8 | 34.6 | 3.0 | 34.6 | 2.8 | 34.6 | 2.5 | 63.9 | 2.0 |
| | 63.9 | 3.0 | | | 63.9 | 2.6 | 63.9 | 2.4 | 63.9 | 2.2 | | |

TABLE XII. Data corresponding to the semidilute solution shear viscosity $\eta$ (in mPa.s) as a function of shear rate $\dot{\gamma}$ (in $s^{-1}$) displayed in Figs 5 (a), (b), (c) and (d) for semidilute polystyrene samples (PS 1.1M and PS 15.4M) at different absolute concentrations $c$ (in g/ml) and at different temperatures $T$ (in °C). Solvent (DOP) viscosities $\eta_s$ (in mPa.s) corresponding to different temperatures are also given.

(a) PS 1.1M, $c = 0.0089$ g/ml

| $T = 22°C$ | | $T = 30°C$ | | $T = 35°C$ | |
|---|---|---|---|---|---|
| $\eta_s = 69.5$ | | $\eta_s = 43.2$ | | $\eta_s = 33.6$ | |
| $\dot{\gamma}$ | $\eta$ | $\dot{\gamma}$ | $\eta$ | $\dot{\gamma}$ | $\eta$ |
| 3.163 | 147.3 | 6.815 | 98 | 6.815 | 74.4 |
| 4.642 | 147.1 | 10 | 97.6 | 10 | 74.7 |
| 6.815 | 146.9 | 14.68 | 97.7 | 14.68 | 74.7 |
| 10 | 147.5 | 21.55 | 97.6 | 21.55 | 74.8 |
| 14.68 | 147.3 | 31.63 | 97.6 | 31.63 | 74.7 |
| 21.55 | 147.2 | 46.43 | 97.7 | 46.43 | 74.6 |
| 31.63 | 147.5 | 68.15 | 97.7 | 68.15 | 74.7 |
| 46.43 | 147.7 | 100 | 97.7 | 100 | 74.7 |
| 68.14 | 147.6 | 146.8 | 97.5 | 146.8 | 74.6 |
| 100 | 147.5 | 215.5 | 96.9 | 215.5 | 74.3 |
| 146.8 | 146.7 | | | | |
| 215.5 | 145.6 | | | | |

(b) PS 15.4M, $c = 0.0027$ g/ml

| $T = 22°C$ | | $T = 30°C$ | | $T = 35°C$ | |
|---|---|---|---|---|---|
| $\eta_s = 69.5$ | | $\eta_s = 43.2$ | | $\eta_s = 33.6$ | |
| $\dot{\gamma}$ | $\eta$ | $\dot{\gamma}$ | $\eta$ | $\dot{\gamma}$ | $\eta$ |
| 2.424 | 113 | 4.642 | 74.1 | 6.813 | 58.3 |
| 3,664 | 111.9 | 6.813 | 74.0 | 10 | 58.3 |
| 5.539 | 112.5 | 10 | 74.0 | 14.68 | 58.5 |
| 8.374 | 111.8 | 14.68 | 73.8 | 21.55 | 58.1 |
| 12,66 | 111.7 | 21.55 | 73.5 | 31.63 | 57.9 |
| 19.14 | 111.2 | 31.62 | 73.1 | 46.42 | 57.4 |
| 28.93 | 110.9 | 46.42 | 72.5 | 68.14 | 57 |
| 43.74 | 109.8 | 68.13 | 72.0 | 100 | 56,5 |
| 66.12 | 108.5 | 100 | 71.6 | 146.8 | 56.1 |
| 99.97 | 107.1 | 146.8 | 71.3 | 215.5 | 56 |

(c) PS 1.1M, $c = 0.0144$ g/ml

| $T = 22°C$ | | $T = 30°C$ | | $T = 35°C$ | |
|---|---|---|---|---|---|
| $\eta_s = 69.5$ | | $\eta_s = 43.2$ | | $\eta_s = 33.6$ | |
| $\dot{\gamma}$ | $\eta$ | $\dot{\gamma}$ | $\eta$ | $\dot{\gamma}$ | $\eta$ |
| 3.161 | 240.1 | 3.161 | 153.4 | 4.64 | 118.1 |
| 4.639 | 240.6 | 4.64 | 153.9 | 6.81 | 118.6 |
| 6.81 | 240.7 | 6.81 | 153.6 | 9.996 | 118 |
| 9.996 | 240 | 9.996 | 153.4 | 14.67 | 118.4 |
| 14.67 | 240.4 | 14.67 | 153.8 | 21.54 | 118.2 |
| 21.54 | 240.5 | 21.54 | 153.8 | 31.61 | 118.4 |
| 31.61 | 240.4 | 31.61 | 153.9 | 46.4 | 118.4 |
| 46.4 | 239.9 | 46.4 | 154 | 68.11 | 118.4 |
| 68.11 | 238.6 | 68.11 | 153.7 | 99.97 | 118.2 |
| 99.97 | 236.5 | 99.97 | 153.1 | 146.7 | 117.6 |
| 146.7 | 233.9 | 146.7 | 152.1 | 215.4 | 116.6 |
| 215.4 | 230.5 | 215.4 | 150.4 | | |

(d) PS 15.4M, $c = 0.0061$ g/ml

| $T = 22°C$ | | $T = 30°C$ | | $T = 35°C$ | |
|---|---|---|---|---|---|
| $\eta_s = 69.5$ | | $\eta_s = 43.2$ | | $\eta_s = 33.6$ | |
| $\dot{\gamma}$ | $\eta$ | $\dot{\gamma}$ | $\eta$ | $\dot{\gamma}$ | $\eta$ |
| 0.999 | 197.2 | 1.584 | 135.1 | 0.999 | 105.1 |
| 1.584 | 196.3 | 2.511 | 133.0 | 1.584 | 104.2 |
| 2.51 | 197.6 | 3.978 | 133.5 | 2.511 | 105.1 |
| 3.978 | 196.6 | 6.307 | 132.7 | 3.979 | 105.8 |
| 6.307 | 195.7 | 9.994 | 132.2 | 6.307 | 104.6 |
| 9.994 | 193.9 | 15.84 | 130.6 | 9.995 | 104.2 |
| 15.84 | 191.7 | 25.11 | 128.3 | 15.84 | 103.2 |
| 25.11 | 189.4 | 39.79 | 126.6 | 25.11 | 101.6 |
| 39.79 | 186.1 | 63.05 | 124.3 | 39.79 | 99.9 |
| 63.05 | 180.3 | 99.96 | 119.7 | 63.06 | 98.1 |
| 99.95 | 176.1 | 158.4 | 115.2 | 99.97 | 95.4 |
| | | | | 158.4 | 91.2 |
| | | | | 251.1 | 86.9 |

TABLE XIII. Data corresponding to the semidilute solution shear viscosity $\eta$ (in mPa.s) as a function of shear rate $\dot{\gamma}$ (in $s^{-1}$) displayed in Figs 5 (e), (f), (g) and (h) for semidilute polystyrene samples (PS 1.1M and PS 15.4M) at different absolute concentrations $c$ (in g/ml) and at different temperatures $T$ (in °C). Solvent (DOP) viscosities $\eta_s$ (in mPa.s) corresponding to different temperatures are also given.

(e) PS 1.1M, $c = 0.0225$ g/ml

| $T = 22$°C, $\eta_s = 69.5$: $\dot{\gamma}$ | $\eta$ | $T = 30$°C, $\eta_s = 43.2$: $\dot{\gamma}$ | $\eta$ | $T = 35$°C, $\eta_s = 33.6$: $\dot{\gamma}$ | $\eta$ |
|---|---|---|---|---|---|
| 0.464 | 506.5 | 3.163 | 309.2 | 4.642 | 238.9 |
| 0.681 | 505.1 | 4.642 | 308.5 | 6.814 | 239.1 |
| 1 | 506 | 6.814 | 308 | 10 | 238.4 |
| 1.468 | 505.4 | 10 | 307.6 | 14.68 | 238.5 |
| 2.155 | 504.9 | 14.68 | 307.9 | 21.55 | 238.3 |
| 3.163 | 505.8 | 21.55 | 307.8 | 31.63 | 238.4 |
| 4.642 | 505.6 | 31.63 | 307.3 | 46.43 | 238 |
| 6.814 | 504.8 | 46.42 | 306.3 | 68.14 | 236.6 |
| 10 | 504.9 | 68.14 | 303 | 100 | 234.1 |
| 14.68 | 504.7 | 100 | 298.7 | 146.8 | 230.3 |
| 21.55 | 502.6 | 146.8 | 292.5 | 215.5 | 225.1 |
| 31.63 | 499.2 | 215.5 | 285.1 | | |
| 46.42 | 492.7 | | | | |
| 68.14 | 483.9 | | | | |
| 100 | 472.9 | | | | |
| 146.8 | 461.4 | | | | |
| 215.5 | 451.6 | | | | |

(f) PS 15.4M, $c = 0.0098$ g/ml

| $T = 22$°C, $\eta_s = 69.5$: $\dot{\gamma}$ | $\eta$ | $T = 30$°C, $\eta_s = 43.2$: $\dot{\gamma}$ | $\eta$ | $T = 35$°C, $\eta_s = 33.6$: $\dot{\gamma}$ | $\eta$ |
|---|---|---|---|---|---|
| 0.251 | 442.2 | 1 | 293 | 1.584 | 223.5 |
| 0.398 | 447.2 | 1.585 | 291.5 | 2.511 | 223.8 |
| 0.631 | 443.7 | 2.512 | 290.6 | 3.98 | 223.4 |
| 0.999 | 442.4 | 3.981 | 285.4 | 6.308 | 217.3 |
| 1.584 | 441.3 | 6.309 | 279.8 | 9.996 | 212.4 |
| 2.51 | 438.6 | 9.994 | 270.5 | 1.84 | 206.9 |
| 3.978 | 426.6 | 15.84 | 263.5 | 25.11 | 200.2 |
| 6.307 | 418.9 | 25.11 | 255.9 | 39.8 | 193.1 |
| 9.995 | 405.4 | 39.79 | 245.5 | 63.07 | 183.3 |
| 15.84 | 397.3 | 63.05 | 228.9 | 99.98 | 169.2 |
| 25.11 | 378.7 | 99.95 | 214.1 | 158.4 | 157.6 |
| 39.79 | 360.4 | | | | |
| 63.05 | 332 | | | | |

(g) PS 1.1M, $c = 0.036$ g/ml

| $T = 22$°C, $\eta_s = 69.5$: $\dot{\gamma}$ | $\eta$ | $T = 30$°C, $\eta_s = 43.2$: $\dot{\gamma}$ | $\eta$ | $T = 35$°C, $\eta_s = 33.6$: $\dot{\gamma}$ | $\eta$ |
|---|---|---|---|---|---|
| 0.316 | 1686.7 | 0.464 | 982.7 | 0.681 | 721 |
| 0.464 | 1687.5 | 0.681 | 980.9 | 1 | 721 |
| 0.681 | 1685.8 | 1 | 983 | 1.468 | 720 |
| 1 | 1686 | 1.467 | 980.9 | 2.154 | 722.8 |
| 1.467 | 1684.4 | 2.154 | 979.1 | 3.161 | 722.2 |
| 2.153 | 1685.1 | 3.162 | 979.4 | 4.64 | 722.2 |
| 3.16 | 1685.4 | 4.64 | 979.9 | 6.81 | 721.9 |
| 4.638 | 1683.5 | 6.811 | 980 | 9.996 | 722 |
| 6.808 | 1676 | 9.997 | 978.8 | 14.67 | 721.2 |
| 9.994 | 1660 | 14.67 | 975.5 | 21.54 | 717.7 |
| 14.67 | 1631.9 | 21.54 | 965.2 | 31.61 | 710.9 |
| 21.53 | 1590.3 | 31.61 | 948.7 | 46.4 | 698.9 |
| 31.6 | 1534.5 | 46.4 | 923.5 | 68.11 | 680.7 |
| 46.39 | 1467.1 | 68.11 | 889.6 | 99.98 | 655.6 |
| 68.08 | 1394.8 | 99.97 | 849.4 | 146.7 | 625.5 |
| 99.93 | 1322.9 | 146.7 | 805 | 215.4 | 591.5 |
| 146.7 | 1255.6 | 215.4 | 759.9 | | |

(h) PS 15.4M, $c = 0.0038$ g/ml

| $T = 22$°C, $\eta_s = 69.5$: $\dot{\gamma}$ | $\eta$ | $T = 30$°C, $\eta_s = 43.2$: $\dot{\gamma}$ | $\eta$ | $T = 35$°C, $\eta_s = 33.6$: $\dot{\gamma}$ | $\eta$ |
|---|---|---|---|---|---|
| 0.251 | 139.7 | 2.512 | 92.0 | 1.585 | 72.6 |
| 0.398 | 139.8 | 3.98 | 91.5 | 2.512 | 72.1 |
| 0.631 | 138.7 | 6.309 | 91.6 | 3.981 | 72.6 |
| 1 | 138.9 | 9.999 | 89.9 | 6.309 | 72 |
| 1.585 | 139.4 | 15.85 | 89.3 | 9.999 | 71.7 |
| 2.512 | 139.3 | 25.12 | 88.1 | 15.85 | 71.2 |
| 3.98 | 139.4 | 39.81 | 87.1 | 25.12 | 70.5 |
| 6.308 | 138.6 | 63.09 | 86.1 | 39.81 | 69.8 |
| 9.998 | 136.9 | 100 | 85.6 | 63.09 | 68.9 |
| 15.85 | 135.5 | | | 100 | 68.1 |
| 25.11 | 134.5 | | | 158.5 | 67.6 |
| 39.8 | 133 | | | | |
| 63.08 | 132.3 | | | | |
